# Supplementary material for: Designing an Automated Vehicle: Strategies for Handling Tasks of a Previously Required Accompanying Person
Source: arXiv:2209.11083 source file (2022-09-22)
Supplement: Supplementary file 1 [file appendix.tex]

%\subsection{Vehicle parameters}
%\label{subsec:vehicleparameters}

\begin{table}[h]
	\centering
	\caption{Vehicle and \todo{tire} parameters}
	\label{tab:vehicleparameters}
	\begin{tabular}{lcS[table-format=3.2]l}
		\toprule
		Parameter		& Symbol							& {Value}	& Unit \\
		\midrule
		Mass			& $m$								& 2200		& \si{\kilogram}\\
		Yaw inertia		& $J_z$								& 2000		& \si{\kilogram\square\meter}\\
		Track width		& $s_\mathrm{l}$, $s_\mathrm{r}$	& 	  .875	& \si{\meter}\\
%						& $s_\mathrm{r}$	& 0.875	& \si{\meter}\\
		Vehicle length	& $l_\mathrm{f}$, $l_\mathrm{r}$	&    1.36	& \si{\meter}\\
%						& $l_\mathrm{r}$	& 1.36	& \si{\meter}\\
		\bottomrule
	\end{tabular}
\end{table}

%
%\subsection{Weights and normalization}
%\label{subsec:weights}

\begin{table}[h]
	\centering
	\caption{Weights and normalization parameters}
	\label{tab:weights}
	\vspace{-.5em}
	\begin{tabular}{cS[table-format=1.2]S[table-format=1.3]S[table-format=1.1]S[table-format=3.2]s[table-unit-alignment = center]}
		\toprule
		\multirow{2}{1.1cm}{Variable}	& \multicolumn{3}{c}{Weights}							& \multicolumn{2}{c}{Normalization}\\
		\cmidrule(lr){2-4} \cmidrule(lr){5-6}
							& $w_{ll}$	& $w_{\mathrm{deg},ll}$	& $w_{\mathrm{f},ll}$ 			& \multicolumn{1}{c}{$\{e_{\mathrm{n},l}\}$}&\multicolumn{1}{c}{$[e_{\mathrm{n},l}]$}\\
		\midrule
		$|v|$				& 0			& {-} 					& 0						& 2		& \meter\per\second\\
		$\dot\psi$			& 1			& {-} 					& 0						& 90	& \degree\per\second\\
		$s$					& 2			& {-} 					& 3						& 1		& \meter\\
		$d$					& 2			& {-} 					& 3						& .4	& \meter\\
		$\psi$				& 0.5		& {-} 					& .3					& 10	& \degree\\
		$\beta$				& 1			& {-} 					& 0						& 45	& \degree\\
		$\delta_{ij}$		& .01		& {-} 					& 0						& 135	& \degree\\
		$\lambda_{ij}$		& .25		& {-} 					& 0						& .08	& \\
		$\dot\delta_{ij}$	& 2			& {-} 					& 0						& 120	& \degree\per\second\\
		$\dot\lambda_{ij}$	& 2			& {-} 					& 0						& .7	& \per\second\\
		$\Delta\delta_i$	& 1			& {-} 					& 0						& 8		& \degree\\
		$\Delta\lambda_j$	& 1			& {-} 					& 0						& 0.05  & \\
		$\alpha_{ij}$		& .3		& {-} 					& 0						& 12	& \degree\\
		$\eta_{ij}$			& .9		& .125					& 0						& 1		&\\
		$\epsilon_\alpha$	& .3		& {-} 					& 0						& 3		& \degree\\
		\bottomrule
	\end{tabular}
\end{table}
%
%
%\subsection{Constraints}
%\label{subsec:constraints}

\begin{table}[h]
	\centering
	\caption{Constraints \todo{Noch mit in vorherige Tabelle einbauen}}
	\label{tab:constraints}
	\begin{tabular}{lccc}
		\toprule
		Parameter			& Symbol 				& Value range							& Unit \\
		\midrule
		Steering angle		& $\delta_{ij}$			& $\left[\num{-30},\num{30}\right]$		& \si{\degree}\\
		Steering rate		& $\dot\delta_{ij}$		& $\left[\num{-120},\num{120}\right]$	& \si{\degree\per\second}\\
		Wheel torque		& $M_{\mathrm{W},ij}$	& $\left[\num{-2000},\num{2000}\right]$	& \si{\newton\meter}\\
		Longitudinal slip	& $\lambda_{ij}$		& $\left[\num{-.12},\num{.12}\right]$	& \\
		Slip angle			& $\alpha_{ij}$			& $\left[\num{-.2},\num{.2}\right]$		& \si{\radian}\\
		\bottomrule
	\end{tabular}
\end{table}
